# Supplementary material for: Derivation of Closed Form of Expected Improvement for Gaussian Process Trained on Log-Transformed Objective
Source: arXiv:2411.18095 source file (2024-11-27)
Supplement: Supplementary file 1 [file appendix-information.tex]

\ifappendix
% include appendix
\clearpage
\appendix
\input{appendices/appendix-full-contents.tex}

\else

% Define the labels in the main sections
\customlabel{data1}{1}
\customlabel{data2}{2}

\fi
